# Supplementary material for: Reasoning Fine-Tuning Induces Persistent Latent Policy States
Source: arXiv:2607.18532 source file (2026-07-20)
Supplement: Supplementary file 1 [file appendix-steering.tex]

\section{Steering Sufficiency Analysis}
\label{app:steering}

% Overall, these results show that input-dependent steering is effective and more controllable on reasoning-distilled models across all three available model pairs (Qwen-1.5B, Llama-8B, Qwen-14B).

\subsection{Steering Results}

Table \ref{tab:all-pairs-steering-summary} shows:
Across all three judged pairs, reasoning checkpoints are easier to steer toward target regimes than base checkpoints.
The effect is strongest on Qwen-1.5B (96.7\% vs 50.0\%), remains clear on Llama-8B (96.7\% vs 85.0\%), and is now also clear on Qwen-14B (97.5\% vs 77.5\%).
Coherence stays high for reasoning sides; on Qwen-14B, coherence separation is especially large (97.5\% vs 66.2\%).

\begin{table}[t]
\centering
\small
\caption{Judge steering/coherence summary by model pair and side.}
\label{tab:all-pairs-steering-summary}
\begin{tabular}{llrrrr}
\toprule
Pair & Side & $N_{\mathrm{judge}}$ & Steer (\%) & Coh. (\%) & Mean conf. \\
\midrule
Qwen-1.5B & Reasoning & 60 & 96.7 & 100.0 & 0.946 \\
Qwen-1.5B & Base      & 60 & 50.0 & 98.3  & 0.911 \\
\midrule
Llama-8B  & Reasoning & 60 & 96.7 & 96.7  & 0.941 \\
Llama-8B  & Base      & 60 & 85.0 & 100.0 & 0.930 \\
\midrule
Qwen-14B  & Reasoning & 80 & 97.5 & 97.5  & 0.940 \\
Qwen-14B  & Base      & 80 & 77.5 & 66.2  & 0.911 \\
\bottomrule
\end{tabular}
\end{table}

\begin{table}[t]
\centering
\small
\caption{Base-minus-reasoning deltas (positive favors base, negative favors reasoning).}
\label{tab:all-pairs-steering-deltas}
\begin{tabular}{lrrr}
\toprule
Pair & $\Delta$Steer (pp) & $\Delta$Coh (pp) & Note \\
\midrule
Qwen-1.5B & -46.7 & -1.7  & Reasoning much easier to steer \\
Llama-8B  & -11.7 & +3.3  & Reasoning steer higher, base coherence slightly higher \\
Qwen-14B  & -20.0 & -31.3 & Reasoning clearly higher steer and coherence \\
\bottomrule
\end{tabular}
\end{table}

\begin{table}[t]
\centering
\small
\caption{High-level pairwise comparison signal.}
\label{tab:all-pairs-highlevel}
\begin{tabular}{p{2.0cm}p{4.0cm}p{4.0cm}p{3.6cm}}
\toprule
Pair & Reasoning-side pattern & Base-side pattern & Comparison outcome \\
\midrule
Qwen-1.5B & Discourse/planning cues align with staged reasoning labels & Mixed numeric/code/noisy tokens & Largest steering gap; strongest reasoning-vs-base separation \\
Llama-8B & More task-structured semantics despite BPE/newline artifacts & More punctuation/glue/format-heavy centroids & Reasoning steerability higher, but coherence close \\
Qwen-14B & Strong reasoning-stage semantics (planning, conditional links, verification, setup) & Mixed computation/final-answer/causal labels with lower coherence under steering & Fully comparable; reasoning outperforms base on both steer and coherence \\
\bottomrule
\end{tabular}
\end{table}

\begin{table}[t]
\centering
\footnotesize
\caption{Aggregate post-activation logit-lens judge metrics (all model--dataset pairs).}
\label{tab:master-triple-four-aggregate}
\setlength{\tabcolsep}{4pt}
\begin{tabularx}{\columnwidth}{>{\raggedright\arraybackslash}X >{\raggedright\arraybackslash}X r r r r r}
\hline
Model & Dataset & HF rows & $N_{\mathrm{judge}}$ & Steer (\%) & Coh. (\%) & Mean conf. \\
\hline
Qwen-1.5B (DeepSeek R1-distill) & GSM8K (\texttt{SDS\_train\_gsm8k}) & 1000 & 300 & 93.7 & 93.7 & 0.93 \\
Qwen-1.5B (DeepSeek R1-distill) & MATH-500 (\texttt{SDS\_math500\_test}) & 1000 & 300 & 98.0 & 98.0 & 0.94 \\
Qwen-1.5B (DeepSeek R1-distill) & MMLU-Pro (\texttt{SDS\_train\_mmlu-pro}) & 1000 & 300 & 91.7 & 96.0 & 0.90 \\
Qwen-1.5B (DeepSeek R1-distill) & SVAMP (\texttt{SDS\_train\_svamp}) & 1000 & 300 & 97.7 & 96.3 & 0.93 \\
Llama-3.1-8B (DeepSeek R1-distill) & GSM8K (\texttt{SDS\_train\_gsm8k}) & 1000 & 300 & 81.3 & 80.7 & 0.92 \\
Llama-3.1-8B (DeepSeek R1-distill) & MATH-500 (\texttt{SDS\_math500\_test}) & 1000 & 300 & 94.3 & 94.7 & 0.93 \\
Llama-3.1-8B (DeepSeek R1-distill) & MMLU-Pro (\texttt{SDS\_train\_mmlu-pro}) & 1000 & 300 & 81.0 & 77.3 & 0.91 \\
Llama-3.1-8B (DeepSeek R1-distill) & SVAMP (\texttt{SDS\_train\_svamp}) & 1000 & 300 & 79.7 & 80.3 & 0.92 \\
Qwen-14B (DeepSeek R1-distill) & GSM8K (\texttt{SDS\_train\_gsm8k}) & 1000 & 300 & 98.0 & 98.7 & 0.94 \\
Qwen-14B (DeepSeek R1-distill) & MATH-500 (\texttt{SDS\_math500\_test}) & 1000 & 300 & 94.7 & 93.0 & 0.94 \\
Qwen-14B (DeepSeek R1-distill) & MMLU-Pro (\texttt{SDS\_train\_mmlu-pro}) & 1000 & 300 & 96.0 & 95.3 & 0.93 \\
Qwen-14B (DeepSeek R1-distill) & SVAMP (\texttt{SDS\_train\_svamp}) & 1000 & 300 & 99.3 & 99.0 & 0.95 \\
\hline
\end{tabularx}
\end{table}

%%%%%%%%%%%%
% runs_persist_chunk_three_scales_hs500_jm300_20260331_003247

\subsection*{GSM8K}
\begin{table*}[t]
\centering
\footnotesize
\caption{Persist-chunk judge: three scales on GSM8K. $\Delta_{\mathrm{steer}}$ = B\% $-$ R\% (steering success).}
\label{tab:persist-three-scales-gsm8k}
\begin{tabular}{@{}lccccccc@{}}
\hline
Family & R steer & B steer & $\Delta_{\mathrm{steer}}$ & R coh & B coh & R min $1{-}c$ & B min $1{-}c$ \\
\hline
Qwen-1.5B & 86.3 & 87.7 & 1.3 & 97.0 & 97.7 & 0.757 & 0.364 \\
Llama-8B & 71.3 & 0.0 & -71.3 & 99.0 & 87.7 & 0.954 & 1.000 \\
Qwen-14B & 79.7 & 78.7 & -1.0 & 96.7 & 97.3 & 0.931 & 0.954 \\
\hline
\end{tabular}
\end{table*}

\subsection*{MATH-500}
\begin{table*}[t]
\centering
\footnotesize
\caption{Persist-chunk judge: three scales on MATH-500. $\Delta_{\mathrm{steer}}$ = B\% $-$ R\% (steering success).}
\label{tab:persist-three-scales-math500}
\begin{tabular}{@{}lccccccc@{}}
\hline
Family & R steer & B steer & $\Delta_{\mathrm{steer}}$ & R coh & B coh & R min $1{-}c$ & B min $1{-}c$ \\
\hline
Qwen-1.5B & 48.0 & 83.7 & 35.7 & 99.0 & 96.7 & 0.501 & 1.017 \\
Llama-8B & 90.0 & 94.7 & 4.7 & 99.0 & 94.7 & 1.053 & 0.780 \\
Qwen-14B & 87.3 & 70.0 & -17.3 & 99.0 & 98.0 & 0.837 & 0.897 \\
\hline
\end{tabular}
\end{table*}

\subsection*{MMLU-Pro}
\begin{table*}[t]
\centering
\footnotesize
\caption{Persist-chunk judge: three scales on MMLU-Pro. $\Delta_{\mathrm{steer}}$ = B\% $-$ R\% (steering success).}
\label{tab:persist-three-scales-mmlupro}
\begin{tabular}{@{}lccccccc@{}}
\hline
Family & R steer & B steer & $\Delta_{\mathrm{steer}}$ & R coh & B coh & R min $1{-}c$ & B min $1{-}c$ \\
\hline
Qwen-1.5B & 83.3 & 63.7 & -19.7 & 93.0 & 92.3 & 0.722 & 1.000 \\
Llama-8B & 90.7 & 1.0 & -89.7 & 98.7 & 93.3 & 0.877 & 0.615 \\
Qwen-14B & 99.0 & 99.0 & 0.0 & 97.3 & 78.3 & 0.973 & 0.866 \\
\hline
\end{tabular}
\end{table*}

\subsection*{SVAMP}
\begin{table*}[t]
\centering
\footnotesize
\caption{Persist-chunk judge: three scales on SVAMP. $\Delta_{\mathrm{steer}}$ = B\% $-$ R\% (steering success).}
\label{tab:persist-three-scales-svamp}
\begin{tabular}{@{}lccccccc@{}}
\hline
Family & R steer & B steer & $\Delta_{\mathrm{steer}}$ & R coh & B coh & R min $1{-}c$ & B min $1{-}c$ \\
\hline
Qwen-1.5B & 51.7 & 68.3 & 16.7 & 97.3 & 98.3 & 1.000 & 0.522 \\
Llama-8B & 78.7 & 0.0 & -78.7 & 97.7 & 87.0 & 0.967 & 1.000 \\
Qwen-14B & 90.7 & 14.0 & -76.7 & 97.3 & 97.7 & 0.997 & 0.818 \\
\hline
\end{tabular}
\end{table*}

%%%%%%%%%%%%
% runs_persist_chunk_batch_qwen14b_20260330_212433

\paragraph{GSM8K --- state labels (persist-chunk LLM).}
\emph{k=0:} Performing basic arithmetic and setting up equations.
\emph{k=1:} Performing basic arithmetic and interpreting problem details.
\emph{k=2:} Performing step-by-step arithmetic calculations.
\emph{k=3:} Performing basic arithmetic calculations.
